# Supplementary material for: On the Topology Awareness and Generalization Performance of Graph Neural Networks
Source: arXiv:2403.04482 source file (2024-07-08)
Supplement: Supplementary file 1 [file appendix_local_structure_proof.tex]

\section{Proof of Theorem~\ref{prop:local_structure}} \label{appendix:local_structure}
In this appendix, we provide proof for Theorem~\ref{prop:local_structure}. Before diving into the detailed proof, we present an outline of the structure of the proof and prove a lemma which we use in the proof of the theorem.

{\bf Outline of the proof for the thereom}
	\begin{enumerate}
		\item By Assumption~\ref{assp:separability} and the premise of the theorem, each vertex would have a unique representation.
            \item Then, by the universal approximation power of neural network, so long there are enough parameters/weights, there exist a prediction head that can map the representation of the vertices to the correct label.
		\item This means that minimum (small) loss is achieved on the vertices in the training set. Since loss function is lower bounded, then there exist a local region around each vertex in the training set that admit monotonic behavior.
	\end{enumerate}

We begin with proving the following lemma about loss value of vertices in the training set with universal approximation power of (ReLu) neural network.

\begin{lemma}\label{lemma:well_train}
 Let $\mathcal{D}$ be a given training set satisfying Assumption~\ref{assp:separability}. Let $\gnnModel$ be a GNN model with injective layer(s), and $f$ be a prediction function with sufficient weights. Then there exist a set of parameters $\theta_{\mathcal{D}}$ such that for any $\epsilon>0$ and $v \in \mathcal{D}$, we have
	$ \loss(f(\gnnModel_{\theta_{\mathcal{D}}}(v))) < \epsilon.$
\end{lemma}

The proof for Lemma~\ref{lemma:well_train} is mainly the application of the Assumption~\ref{assp:separability} and {\bf Theorem 1} in~\citep{memorization}. We start with restating the {\bf Theorem 1} in~\citep{memorization}.

\begin{theorem}\label{thm:uni_approx}
    There exists a two-layer neural network with ReLU activations and $2n+d$ weights that can represent any function on a sample of size $n$ in $d$ dimensions.
\end{theorem}

The proof of Theorem~\ref{thm:uni_approx} can be found in~\cite{memorization}. Other universal approximation theorem can be used to replace Theorem~\ref{thm:uni_approx}. 

\begin{proof}
  Let $\mathcal{D}$ be the training set of size $n$. By Assumption~\ref{assp:separability}, we know there is no identical inputs to the GNN in the training set. By the injective property assumed on the GNN layers, the learnt representation for all the vertex in the training are different. In other word, $\forall v, u \in \mathcal{D}$, we have that $h_u \neq h_v \in \mathds{R}^d$, where $d$ is the dimension of the embedding space. Let $\mathcal{H}_{\mathcal{D}}$ be the set of representation of the training set. It is easy to construct a mapping function $g$ that take each representation in $\mathcal{H}_{\mathcal{D}}$ to its corresponding label. By Theorem~\ref{thm:uni_approx}, the prediction $f$ can approximate $g$ arbitrarily well with a two-layer neural network of Relu activation and $2n+d$ weights.
\end{proof}

Proof for Theorem~\ref{prop:local_structure}.
\begin{proof}
  Let $\theta_D$ be the set of parameters learnt by the GNN model and $f$ be prediction head function
  that satisfy properties given in Lemma~\ref{lemma:well_train}. Namely, for each vertex $v \in D$ and any $\epsilon > 0$, we have that
  
  $$\loss_{\theta_D}(f(h_v)) < \epsilon,$$
  where $h_v = \gnnModel(v)$. This means that $\loss_{\theta_D}(f(h_v)) \mapsto 0$ and we know that the $\loss$ function is a continuous function of range $\mathds{R}_+$. $\loss_{\theta_D}(f(h_v))$ achieves the global minimum of the loss function in the embedding space.

  By Assumption~\ref{assp:local_curvation}, we know that $\frac{d}{dh}\loss (f(h_v))$ and $\frac{d^2}{d^2h}\loss (f(h_v))$ exist. This implies that 
  
  $$\frac{d}{dh}\loss (f(h_v)) = 0,$$
  
  as this is the necessary condition for $h_v$ to achieve a local minimum. Furthermore, as $\loss_{\theta_D}(f(h_v))$ also achieves the global minimum, this implies that
  
  $$\frac{d^2}{d^2h}\loss (f(h_v)) \geq 0.$$

  This means that there must exist a $r_v > 0$ such that $\forall h \in N_{r_v}(h_v) \subset \embdingSpace$, we have
  
  $$\frac{d}{dh}\loss (f(h_v)) \geq 0.$$ 
  
  For $d(h,h_v) \leq d(h',h_v) \leq r_v$, we can rewrite $h' = h + d$. Then we have,
  
  \begin{equation*}
  \begin{split}
      \loss (f(h')) =  \loss (f(h + d))\\
      \geq \loss (f(h)) + \frac{d}{dh}\loss (f(h)) \|d\|
  \end{split}
  \end{equation*}
 
 Because $ \frac{d}{dh}\loss (f(h)) \geq 0$ and $\|d\| > 0$, we have that  
 $$\loss (f(h')) > \loss (f(h)).$$
\end{proof}
