# Supplementary material for: On the Topology Awareness and Generalization Performance of Graph Neural Networks
Source: arXiv:2403.04482 source file (2024-07-08)
Supplement: Supplementary file 2 [file appendix_max_cover.tex]

\section{Maximum Cover and Sampling Procedure}\label{appendix:max_cover}
In this appendix we provide a detailed reduction of optimization (\ref{eq:max_cover}) to the maximal coverage problem. 

% \begin{comment}
% First recall the formulation of optimization (\ref{eq:max_cover}).

% \begin{equation}
% 	\begin{split}
% 		& \max_{D \subset V} \sum_{u \in V\setminus D} I_r(u|D) \\
% 		s.t.& ~~~ |D| \leq k\\
% 	\end{split}
% \end{equation}
% where $k$ is the given initial set size and $r$ is the given neighborhood radius. $I_r(u|D)$ is an indicator function: $I_r(u|D) = 1$ if there exists a vertex $v \in D$ such that $u \in N_r(v)$, and $I_r(u|D) =0$, otherwise. 
% \end{comment}
Let's create binary variables $X_v$  and $y_v$ for each vertex $v \in V$ such that $X_v$ indicates whether vertex $v$ is selected in the cover and $y_v$ indicates whether vertex $v$ is covered by some neighborhood of vertex in the selected set. We can rewrite optimization (\ref{eq:max_cover}) as follows: 

\begin{equation}\label{eq:max_cover_sd}
	\begin{split}
		& \max \sum_{v \in V} y_v\\
		s.t.&~~~  \sum_{v \in V} X_v \leq k\\
		    & \sum_{u \in N_r(v)} X_u \geq y_v,\forall v \in V \\
		    & y_v \in \{0,1\}\\
		    & X_v \in \{0,1\}
	\end{split}
\end{equation}
$\sum_{v \in V} X_v \leq k$ ensures no more than $k$ vertexes are selected into the set. $\sum_{u \in N_r(v)} X_u \geq y_v,\forall v \in V$ ensures that $y_v$ is $1$ if and only if vertex $v$ is covered by the neighborhood of some vertex $u$ selected in the cover. The objective function is to maximize the number of vertexes covered. Optimization (\ref{eq:max_cover_sd}) has the standard form of maximal coverage problem as presented in~\citep{approx}. Therefore, we can directly employ the heuristic algorithm and its performance guarantee in~\citep{approx}.

\begin{algorithm}[!h]
  \caption{Coverage-based Sampling}
  \label{alg:coverage_based_sampling}
\begin{algorithmic}
  \STATE {\bfseries Input:} $D \subset V$ //labelled set \\
  \REQUIRE $\mathcal{G}$ //graph\\
  \REQUIRE $k$ //size of set to be sampled\\
  \REQUIRE $r$ //coverage radius\\
  
  Sample/select the set of size $k$ with the following procedures:
  \begin{enumerate}[leftmargin=.5in]
       \item initial each vertex in the graph with an uncovered status
      \item initialize each vertex $v \in D$ with $p_v$ with its $| \mathcal{N}_r(u)|$
      \item sample $u$ from $D$ based on probability proportion to $p_u$ (e.g., normalized each $p_u$ with the total some $\sum_{v \in D} p_v$)
      \item flag the vertices in the neighbourhood $\mathcal{N}_r(u)$ as covered status
      \item update each remaining vertex $v \in D \setminus \{u\}$ with number of uncovered vertices in $\mathcal{N}_r(v)$
      \item repeat until $k$ vertices are sampled
  \end{enumerate}
\end{algorithmic}
\end{algorithm}
