# Supplementary material for: On the Topology Awareness and Generalization Performance of Graph Neural Networks
Source: arXiv:2403.04482 source file (2024-07-08)
Supplement: Supplementary file 3 [file appendix_partial_cover.tex]

\section{Partial Cover}\label{appendix:partial_cover}
In this appendix we provide a detailed reduction of optimization (\ref{eq:partial_cover}) to the partial coverage problem. 

\begin{comment}
First recall the formulation of optimization (\ref{eq:partial_cover}).

\begin{equation}
	\begin{split}
		& \min_{D \subset V} |D| \\
		s.t.&   \sum_{u \in V-D} I_r(u|D)  \geq g |V| \\
	\end{split}
\end{equation}

where $g \in [0,1]$ and $I_r(u|D)$ is an indicator function: $I_r(u|D) = 1$ if there exists a vertex $v \in D$ such that $u \in N_r(v)$, and $I_r(u|D) =0$, otherwise. 
\end{comment}
Let's create binary variables $X_v$  and $y_v$ for each vertex $v \in V$ suc that $X_v$ indicates whether vertex $v$ is selected in the cover and $y_v$ indicates whether vertex $v$ is covered by neighborhood of some vertex in the selected set. We can rewrite optimization (\ref{eq:partial_cover}) above as follows:

\begin{equation}\label{eq:partial_cover_sd}
	\begin{split}
		& \min \sum_{v \in V} X_v\\
		s.t.& \sum_{u \in N_r(v)} X_u \geq y_v,\forall v \in V \\
		    & \sum_{v \in V} y_v \geq g |V|\\
		    & y_v \in \{0,1\}\\
		    & X_v \in \{0,1\}
	\end{split}
\end{equation}
 $\sum_{u \in N_r(v)} X_u \geq y_v,\forall v \in V$ ensures that $y_v$ is $1$ if and only if vertex $v$ is covered by the neighborhood of some vertex $u$ selected in the cover. $\sum_{v \in V} y_v \geq g |V|$ ensures that there are at least $g |V|$ number of vertexes covered. The objective function is to minimize the number of vertex selected in the cover set. Optimization (\ref{eq:partial_cover_sd}) has the standard form of partial coverage problem as presented in~\citep{partial_cover} and therefore, we can directly employ the heuristic algorithm and its performance guarantee in~\citep{partial_cover}.
