# Supplementary material for: On the Topology Awareness and Generalization Performance of Graph Neural Networks
Source: arXiv:2403.04482 source file (2024-07-08)
Supplement: Supplementary file 4 [file appendix_trainSet_selection_proof.tex]

\section{Proof of Theorem~\ref{theorem:sub_group_performance}}\label{appendix:trainset_proof}
Before diving into the detailed proof, we present an outline of the structure of the proof and prove a lemma which we use in the proof of the theorem.

{\bf Outline of the proof for the thereom}
	\begin{enumerate}
		\item Suppose we are given $T$ and $T'$, two test groups which satisfy the premise of the theorem;
		\item Then, we can approximate and bound the loss of each vertex in these group based on the nearest vertex in the training set by extending the result from Theorem~\ref{prop:local_structure};
		\item Based on smoothness of curvature assumed in Assumption~\ref{assp:local_curvation}, we can bound the behavior of vertexes in the test set and derive the desired result.
	\end{enumerate}
	
\begin{lemma}\label{lemma:non_intersecting_local}
    Let $D$ be a given training set. $\gnnModel$ and $f$ are the GNN model and prediction function which have parameter $\theta$ and satisfy the property in Lemma~\ref{lemma:well_train}. Let $u, v$ be two arbitrary vertexes in $D$ with representations $h_u = \gnnModel(u)$ and $h_v = \gnnModel(v)$. Let $N_{r_v}(h_v)$ and $N_{r_u}(h_u)$ be the neighborhood %simple region
    given in Proposition~\ref{prop:local_structure}. Furthermore, let $N_{r_v,+}(h_v) := \{h \in N_{r_v}(h_v)| \loss(f(h)) > 0 \}$, %\cwu{it should be $N_{r_v,+}(h_v) := \{h \in N_{r_v}(h_v)|\loss(f(h))>0 \}$?}, 
    i.e., the set whose elements have positive loss values. $N_{r_u,+}(h_u)$ is Similarly defined. Then, we have that 
    $$N_{r_u,+}(h_u) \cap N_{r_v,+}(h_v) = \emptyset.$$
\end{lemma}

\begin{proof}
    Suppose the opposite: there exists $h$ which belongs to $N_{r_u,+}(h_u)$ and  $N_{r_v,+}(h_v)$ at the same time. In other words, 
    $$ h \in  N_{r_v,+}(h_v) \cap N_{r_u,+}(h_u).$$ %\cwu{$N_{r_v,+}(h_v)\cap N_{r_u,+}(h_u)$?}
    
    By their definition, % of $N_{r_v,+}(h_v)$ and $N_{r_v,+}(h_v)$, 
    $N_{r_v,+}(h_v)$ and $N_{r_u,+}(h_u)$ are open sets. By definition of an open set, there exist $r_{h,v}$ and $r_{h,u}$ such that the neighborhood $N_{r_{h,v}}(h) \subseteq N_{r_v}(h_v)$ %\cwu{$\subseteq$?} 
    and the neighborhood $N_{r_{h,u}}(h) \subseteq N_{r_u}(h_u)$ %\cwu{$\subseteq$?}. 
    
    Let $r_h = \min\{r_{h,v}, r_{h,u}\}$. We have that neighborhood $N_{r_{h}}(h)$ are in both $N_{r_u}(h_u)$ and $N_{r_v}(h_v)$.
    
    Consider $h' \in N_{r_{h}}(h)$ such that 
    $$d(h,h_v) < d(h',h_v),$$ 
    and 
    $$d(h,h_u) > d(h',h_u).$$
    Such $h'$ exists because $h_v$ and $h_u$ are two distinct points in the embedding space. Next, let's consider the loss value of $h,h'$ from the perspective of $h_v$. Because 
    $$d(h,h_v) < d(h',h_v),$$ 
    by Proposition~\ref{prop:local_structure}, we have that
    $$\loss(f(h)) < \loss(f(h')).$$
    Similarly, if consider the loss value of $h,h'$ from the perspective of $h_u$, we have that
    $$\loss(f(h)) > \loss(f(h')),$$
    because $$d(h,h_u) > d(h',h_u).$$ 
    We reach a contradiction.
\end{proof}
Lemma~\ref{lemma:non_intersecting_local} implies that each vertex can be in at most one of these neighborhoods %simple region 
at a time. Next, we provide the proof for Theorem \ref{theorem:sub_group_performance}. 

\begin{proof}
Let $G = (V, E)$ be the input graph with node feature vector $X_v$ for all $v \in V$. Let $D \subset V$ be the training sets.  Let $\gnnModel $ be a given GNN model. Let $f$ be the prediction function that maps the output of $\gnnModel$ to the class representation.  Let $\loss$ be the loss function with range $\mathds{R}_+$. Let $\theta_{D}$ be the sets of model parameters learnt using training set $D$, which satisfy Lemma~\ref{lemma:well_train}. In other words, we have,

	\begin{equation}
    	\sum_{u \in D} \loss (f (\gnnModel_{\theta_{D}}(u)))  = 0
	\end{equation}
	
Let $T,T'$ be the two test groups satisfy the premise of the theorem. We have a one-to-one mapping $g:T \mapsto T'$. Now, let's consider the loss on the test set $T$ with the model $\gnnModel_{D}$, which can be written as:

    \begin{equation}
        \sum_{u \in T} \loss (f(\gnnModel_{\theta_D}(u)))
    \end{equation}

By premise,  we have that for each $u \in T$, there exists at least one $v \in D$ such that $\gnnModel(u) \in N_{r_v}(\gcnModel(v))$ where $N_{r_v}(\gcnModel(v))$ satisfies properties of Proposition~\ref{prop:local_structure}. In other words, the loss function is monotonically increasing with respect to the embedding distance in $N_{r_v}(\gcnModel(v))$. 

By Lemma~\ref{lemma:non_intersecting_local}, we know that $u$ can be in only one of this neighborhoods. Let $Q: T \mapsto D$ be the mapping that maps vertex $u \in T$ to its corresponding simple neighborhood that is centered at a vertex $Q(u) \in D$. For simplicity, we denote the vertex as $q_u = Q(u)$.  Due to Proposition~\ref{prop:local_structure} and Assumption~\ref{assp:local_curvation}, we can do a quadratic approximation of $u$ around $q_u$ and have the following upper bound:

\begin{equation}\label{eq:quadratic_approximation}
\begin{split}
        \loss (f(\gnnModel_{\theta_D}(u))) & \leq  \loss (f(\gnnModel_{\theta_D}(q_u)))+ \langle \gnnModel_{\theta_D}(u)-\gnnModel_{\theta_D}(q_u), D \gnnModel_{\theta_D}(q_u) \rangle\\
        & + \frac{M_{u}}{2}\|\gnnModel_{\theta_D}(u)-\gnnModel_{\theta_D}(q_u)\| \\
\end{split}
\end{equation}

where $$M_u = \sup \{ D^2 \loss(f(h))| h \in N_{r_{q_u}}(q_u)  \},$$
and
$$r_{q_u} = \|q_u - u\|.$$

Let 
\begin{equation}
    M^*_{D} = \max \{ \|M_u\| | u \in T \}
\end{equation}

$M^*_{D}$ exists since $T$ is finite. Then, we obtain the following upper bound that is universal for all vertexes in $T$: 

\begin{equation} \label{eq:upper}
    \sum_{u \in T} \loss (f(\gnnModel_{\theta_D}(u))) \leq \sum_{u \in T} L_1(u) + \frac{M^*_{D}}{2}\|\gnnModel_{\theta_u}(u)-\gnnModel_{\theta_D}(q_u)\|
\end{equation}

where $$L_1(u) = \loss (f(\gnnModel_{\theta_D}(q_u)))+ \langle \gnnModel_{\theta_u}(u)-\gnnModel_{\theta_D}(q_u), D \gnnModel_{\theta_D}(q_u) \rangle.$$ 

Similarly, let $Q': T' \mapsto D$ be the mapping that maps vertex $u \in T'$ to its corresponding simple neighborhood that is centered at a vertex $Q'(u) \in D$. For simplicity, we denote the vertex as $q'_u = Q'(u)$.  Again, due to Proposition~\ref{prop:local_structure} and Assumption~\ref{assp:local_curvation}, we can do a quadratic approximation of $u$ around $q'_u$ and have the following lower bound:

\begin{equation}\label{eq:quadratic_approximation_lower}
\begin{split}
        \loss (f(\gnnModel_{\theta_D}(u))) & \geq  \loss (f(\gnnModel_{\theta_D}(q'_u)))+ \langle \gnnModel_{\theta_D}(u)-\gnnModel_{\theta_D}(q'_u), D \gnnModel_{\theta_D}(q'_u) \rangle\\
        & + \frac{L_{u}}{2}\|\gnnModel_{\theta_D}(u)-\gnnModel_{\theta_D}(q'_u)\| \\
\end{split}
\end{equation}

where $$L_u = \inf \{ D^2 \loss(f(h))| h \in N_{r_{q_u'}}(q_u')  \},$$
and
$$r_{q_u'} = \|q_u' - u\|.$$

Let 
\begin{equation}
    L^*_{D} = \min \{ \|L_u\| | u \in T' \}
\end{equation}

$L^*_{D}$ exists since $T'$ is finite. Then, we obtain the following lower bound that is universal for all the vertexes in $T'$:

\begin{equation} \label{eq:lower}
    \sum_{u \in T'} \loss (f(\gnnModel_{\theta_D}(u))) \geq \sum_{u \in T'} L_1'(u) + \frac{L^*_{D}}{2}\|\gnnModel_{\theta_D}(u)-\gnnModel_{\theta_D}(q'_u)\|
\end{equation}

where $$L_1'(u) = \loss (f(\gnnModel_{\theta_D}(q'_u)))+ \langle \gnnModel_{\theta_D}(u)-\gnnModel_{\theta_D}(q'_u), D \gnnModel_{\theta_D}(q'_u) \rangle.$$ 

For simplicity, suppose the cardinality of $T$ and $T'$ are $k$, and let $I = \{1,...,k\}$. 

Let's consider the difference between \eqref{eq:lower} and \eqref{eq:upper}:
\begin{equation}
    \begin{split}
         & \sum_{u \in T'} \loss (f(\gnnModel_{\theta_D}(u)))) -  \sum_{u \in T}  \loss (f(\gnnModel_{\theta_D}(u))) \\
         &= \sum_{i \in I} \loss (f(\gnnModel_{\theta_D}(v_i))) - \loss (f(\gnnModel_{\theta_D}(u_i)))\\
         & > \sum_{i \in I} L_1'(v_i) + \frac{L^*_{D}}{2}\|\gnnModel_{\theta_D}(v_i) - \gnnModel_{\theta_D}(q'_{v_i})\| - L_1(u_i) - \frac{M^*_{D}}{2}\|\gnnModel_{\theta_D}(u_i)-\gnnModel_{\theta_D}(q_{u_i})\| \\
         & = \sum_{i \in I} (L_1'(v_i) - L_1(u_i)) + \sum_{i \in I} \big[ \frac{L^*_{D}}{2}\|\gnnModel_{\theta_D}(v_i) - \gnnModel_{\theta_D}(q'_{v_i})\| -  \frac{M^*_{D}}{2}\|\gnnModel_{\theta_D}(u_i)-\gnnModel_{\theta_D}(q_{u_i})\| \big]\\
         & =  \sum_{i \in I} (L_1'(v_i) - L_1(u_i)) + \\
         & \frac{L^*_{D}}{2} \sum_{i \in I}  \big[\|\gnnModel_{\theta_D}(v_i)-\gnnModel_{\theta_D}(q'_{v_i})\| \big] - \frac{M^*_{D}}{2} \sum_{i \in I}  \big[ \|\gnnModel_{\theta_D}(u_i)-\gnnModel_{\theta_D}(q_{u_i})\|\big]
    \end{split}
\end{equation}

Since $q_{u_i}$ and $q'_{v_i}$ are local/global minima of the loss function,  we get that 
$$L_1'(v_i) = L_1(u_i).$$

This leads to that
\begin{equation}\label{eq:intermediate_diff}
    \begin{split}
         & \sum_{i \in I} \loss (f(\gnnModel_{\theta_D}(v_i))) - \loss (f(\gnnModel_{\theta_D}(u_i))) \\
         & >  \frac{L^*_{D}}{2} \sum_{i \in I} \big[\|\gnnModel_{\theta_D}(v_i)-\gnnModel_{\theta_D}(q'_{v_i})\| \big] - \frac{M^*_{D}}{2} \sum_{i \in I} \big[ \|\gnnModel_{\theta_D}(u_i)-\gnnModel_{\theta_D}(q_{u_i})\|\big]
    \end{split}
\end{equation}

To simplify the notation, let's denote 
$$S = \sum_{i \in I} \big[ \|\gnnModel_{\theta_D}(u_i)-\gnnModel_{\theta_D}(q_{u_i})\|\big],$$
$$S' =\sum_{i \in I} \big[\|\gnnModel_{\theta_D}(v_i)-\gnnModel_{\theta_D}(q'_{v_i})\| \big].$$
and
$$W = \sum_{i \in I}  d(u_i,D) ,$$
$$W' = \sum_{i \in I}  d(v_i,D) $$

By Definition~\ref{def:distortion}, we have that
$$r W \leq S \leq \alpha r W, $$
and
$$r W' \leq S' \leq \alpha r W'.$$

Then, we can rewrite \eqref{eq:intermediate_diff} as follows:
\begin{equation}\label{eq:intermediate_diff2}
    \begin{split}
         & \sum_{i \in I} \loss (f(\gnnModel_{\theta_D}(v_i))) - \loss (f(\gnnModel_{\theta_D}(u_i))) \\
         & >   \frac{L^*_{D}}{2} S' - \frac{M^*_{D}}{2} S.
    \end{split}
\end{equation}

Since $M^*_{D}> L^*_{D} > 0$, let $\beta = \frac{M^*_{D}}{L^*_{D}}$.

Similarly, By the premise of the theorem, we have that, 
$$S' \geq rW' > \alpha r W \geq  S.$$

Let $\gamma = \frac{S'}{S}.$ We can obtain the following bound on $\gamma$,

\begin{equation}
    \begin{split}
    \gamma  & = \frac{S'}{S}\\
            & \geq \frac{rW'}{\alpha r W}\\
            & \geq \frac{1}{\alpha} \frac{W'}{W} \\
            & \geq \frac{1}{\alpha} \alpha \delta \\
            & \geq \delta
    \end{split}
\end{equation}

Substituting the above results into \eqref{eq:intermediate_diff2}, we get that 

\begin{equation}\label{eq:intermediate_diff3}
    \begin{split}
    & \frac{1}{2} \big[L^*_{D} S' - M^*_{D} S \big]\\
    & = \frac{1}{2} \big[L^*_{D}  \gamma S - \beta L^*_{D} S\big]  \\
    & \geq \frac{1}{2} L^*_{D} S (\delta- \beta)
    \end{split}
\end{equation}

Therefore, if $\delta >  \beta =  \frac{M^*_{D}}{L^*_{D}}$, then we have that

\begin{equation}
    \begin{split}
       & \frac{1}{2} \big[L^*_{D} S' - M^*_{D} S \big] > 0,
    \end{split}
\end{equation}

leading to,

\begin{equation}
    \begin{split}
        \sum_{u \in T'} \loss (f(\gnnModel_{\theta_D}(u)))) -  \sum_{u \in T}  \loss (f(\gnnModel_{\theta_D}(u))) > 0
    \end{split}
\end{equation}

This completes the proof for Theorem \ref{theorem:sub_group_performance}.

\end{proof}
