# Supplementary material for: On the Topology Awareness and Generalization Performance of Graph Neural Networks
Source: arXiv:2403.04482 source file (2024-07-08)
Supplement: Supplementary file 7 [file lemma_non_intersecting_local_neighbor.tex]

\begin{lemma}\label{lemma:non_intersecting_local}
    Let $D$ be a given training set. $\gnnModel$ and $f$ are the GNN model and prediction function which have parameter $\theta$ and satisfy the property in Lemma~\ref{lemma:well_train}. Let $u, v$ be two arbitrary vertexes in $D$ with representations $h_u = \gnnModel(u)$ and $h_v = \gnnModel(v)$. Let $N_{r_v}(h_v)$ and $N_{r_u}(h_u)$ be the neighborhood %simple region
    given in Proposition~\ref{prop:local_structure}. Furthermore, let $N_{r_v,+}(h_v) := \{h \in N_{r_v}(h_v)| \loss(f(h)) > 0 \}$, %\cwu{it should be $N_{r_v,+}(h_v) := \{h \in N_{r_v}(h_v)|\loss(f(h))>0 \}$?}, 
    i.e., the set whose elements have positive loss values. $N_{r_u,+}(h_u)$ is Similarly defined. Then, we have that 
    $$N_{r_u,+}(h_u) \cap N_{r_v,+}(h_v) = \emptyset.$$
\end{lemma}

\begin{proof}
    Suppose the opposite: there exists $h$ which belongs to $N_{r_u,+}(h_u)$ and  $N_{r_v,+}(h_v)$ at the same time. In other words, 
    $$ h \in  N_{r_v,+}(h_v) \cap N_{r_u,+}(h_u).$$ %\cwu{$N_{r_v,+}(h_v)\cap N_{r_u,+}(h_u)$?}
    
    By their definition, % of $N_{r_v,+}(h_v)$ and $N_{r_v,+}(h_v)$, 
    $N_{r_v,+}(h_v)$ and $N_{r_u,+}(h_u)$ are open sets. By definition of an open set, there exist $r_{h,v}$ and $r_{h,u}$ such that the neighborhood $N_{r_{h,v}}(h) \subseteq N_{r_v}(h_v)$ %\cwu{$\subseteq$?} 
    and the neighborhood $N_{r_{h,u}}(h) \subseteq N_{r_u}(h_u)$ %\cwu{$\subseteq$?}. 
    
    Let $r_h = \min\{r_{h,v}, r_{h,u}\}$. We have that neighborhood $N_{r_{h}}(h)$ are in both $N_{r_u}(h_u)$ and $N_{r_v}(h_v)$.
    
    Consider $h' \in N_{r_{h}}(h)$ such that 
    $$d(h,h_v) < d(h',h_v),$$ 
    and 
    $$d(h,h_u) > d(h',h_u).$$
    Such $h'$ exists because $h_v$ and $h_u$ are two distinct points in the embedding space. Next, let's consider the loss value of $h,h'$ from the perspective of $h_v$. Because 
    $$d(h,h_v) < d(h',h_v),$$ 
    by Proposition~\ref{prop:local_structure}, we have that
    $$\loss(f(h)) < \loss(f(h')).$$
    Similarly, if consider the loss value of $h,h'$ from the perspective of $h_u$, we have that
    $$\loss(f(h)) > \loss(f(h')),$$
    because $$d(h,h_u) > d(h',h_u).$$ 
    We reach a contradiction.
\end{proof}
